# Supplementary material for: Thermal switching of indirect interlayer exchange in magnetic multilayers
Source: arXiv:1705.01056 ancillary file (2017-06-30)
Supplement: Supplementary file 1 [file SupplMater.pdf]

# Thermal switching of indirect interlayer exchange in magnetic multilayers

D. M. Polishchuk, Yu. O. Tykhonenko-Polishchuk, A. F. Kravets, and V. Korenivski

**Supplementary A: Magnetic properties of decoupled Fe(2)/Cr($d_{Cr}$)/Fe(2) trilayers.**

We additionally note that the values of the coercivity field of the top and bottom Fe layers differ somewhat. We have performed magneto-optical Kerr effect (MOKE) measurements with the modulation of the polarization axis done using a photo-elastic modulator (PEM), which allows to selectively study the magnetization of the individual layers in the stack, Fe(2)/Cr(10)/Fe(2). The MOKE data measured on the 1$^{st}$ PEM-harmonic (50 kHz) are insensitive to the inner Fe layer (bottom, grown directly on the substrate), as shown for the reference bilayer Fe(2)/Cr(10) (Fig. A1, black). The 2$^{nd}$ PEM-harmonic (100 kHz) picks up both the top and the bottom Fe layers (Fig. A1, red), which corresponds to the major loop measured with the VSM magnetometer (see main article). Consequently, the 1$^{st}$-harmonic MOKE loop characterizes only the top Fe film, grown on Cr(10), which has lower coercivity than the bottom film grown directly on to Si<100>. This is fully consistent with the MOKE properties of the individual reference samples Fe(2)/Cr(10) and Cr(10)/Fe(2), shown in the inset to Fig. A1. The difference in the coercive field is connected with the specifics of growth of the Fe films on pure Si<100> and relatively thick Cr(10) underlayers. We can thus verify that the two Fe films in the studied stacks are fully decoupled for thicker Cr spacers (>3 nm).

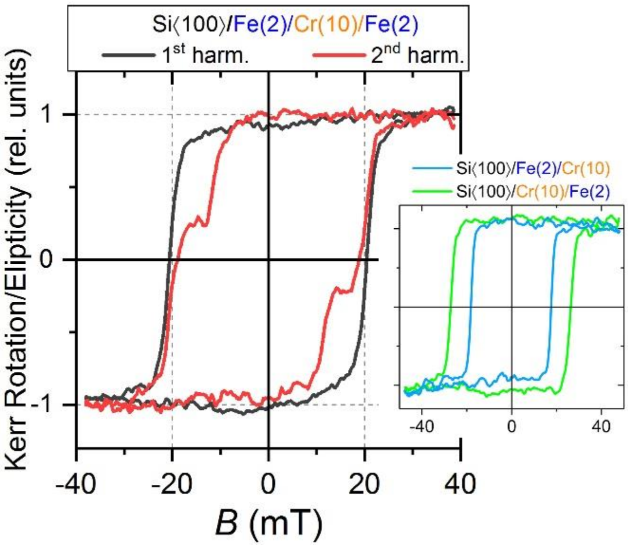


**Figure A1.** 1$^{st}$ and 2$^{nd}$ harmonics PEM-MOKE hysteresis loops for Fe(2)/Cr(10)/Fe(2) trilayer grown on to Si<100> and Si<100>/$SiO_2$. Inset: 2$^{nd}$ harmonic PEM-MOKE loops for Fe(2)/Cr(10) and Cr(10)/Fe(2) bilayers.

**Supplementary B: Magnetic properties of diluted $Fe_xCr_{100-x}$ alloys.**

$Fe_xCr_{100-x}$ alloys with $x$ = 30, 35, and 40 at. % Fe, were obtained by co-deposition from individual Cr and Fe targets. The following experiments were performed to verify that the properties of the $Fe_xCr_{100-x}$ alloy films obtained are essentially those of the bulk alloy.

The alloy with $x$ = 40 % is ferromagnetic at room temperature (RT), which is clear from the hysteresis loop of a 20 nm $Fe_{40}Cr_{60}$ film shown in Fig. B1a. The Curie temperature of this alloy film, $T_C$, is significantly higher than RT. The magnetization of the $Fe_{35}Cr_{65}$ film (also 20 nm thick), is negligible in comparison, below the detection limit of the VSM, though the film should be at the onset of ferromagnetism, with the bulk $T_C$ just above RT.

In order to show that the $Fe_{35}Cr_{65}$ is in the weakly ferromagnetic state, a reference set of tri-layer samples was fabricated, Fe(4)/$Fe_xCr_{100-x}$(20)/Fe(4)/IrMn(10), where the top Fe layer was exchange-pinned by an antiferromagnet (IrMn). The shift of the top-Fe(4) loop due to the pinning is translated to the bottom-Fe(4) layer via the spacer, only if the spacer possesses some degree of magnetic ordering. Fig. B1b shows $M(B)$ for two reference samples, which clearly differ in behavior as regards the spacer-mediated exchange. Thus, for the x = 30 % sample the two Fe loops are fully decoupled indicating a paramagnetic spacer with no interlayer exchange. On the other hand, the un-pinned Fe loop for the sample with the $Fe_{35}Cr_{65}$(20) spacer is shifted in field, which indicates non-zero magnetic ordering in the spacer. We note that the spacer thickness of 20 nm is sufficient for excluding the proximity effects of the two ferromagnetic interfaces (see, e.g., Ref. 31 of the main article).

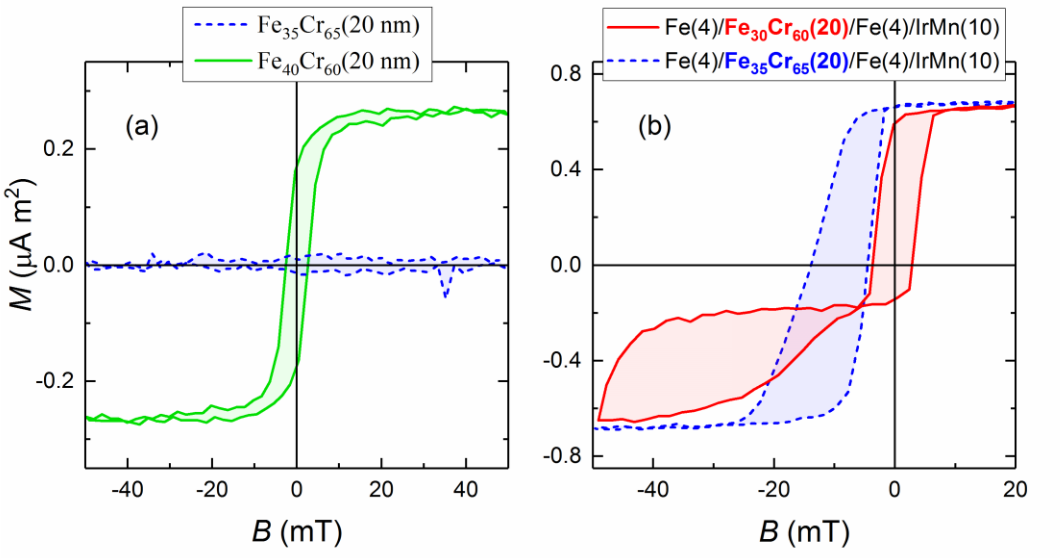


**Figure B1.** Room-temperature VSM magnetization curves for (a) 20-nm thick $Fe_{35}Cr_{65}$ and $Fe_{40}Cr_{60}$ thin films and (b) reference structures Fe(4)/$Fe_xCr_{100-x}$(20)/Fe(4)/IrMn(10), $x$ = 30 and 35 %.

**Supplementary C: Phenomenology of bi-linear exchange coupling.**

A phenomenological magnetostatic model has the following assumptions. First, the magnetic field is applied in the plane of the films, which corresponds to our experiment and simplifies the calculations. Second, the individual grains in the polycrystalline films are characterized by two-fold in-plane anisotropy with the easy axes uniformly distributed across all in-plane angles (the films were deposited under in-plane rotation). These assumptions are reasonable for the studied system and produced the best fit to the measured *M*(*B*) data at various temperatures.

The free energy density for a $FM_1$/NM/$FM_2$ system can then be written as

$$\begin{gathered} U = U_B + U_\mathrm{a} + U_j = \\ = -MB\left[\cos(\varphi_1 - \varphi_B) + \cos(\varphi_2 - \varphi_B)\right] - 1/2\, MB_\mathrm{a}\left[\cos^2\varphi_1 + \cos^2\varphi_2\right] + \\ +1/2\, MB_j \cos(\varphi_1 - \varphi_2), \end{gathered} \tag{C1}$$

where $U_B$, $U_\mathrm{a}$ and $U_j$ are, respectively, the Zeeman energy of the FM layers in field **B** = ($B$, $\varphi_B$), uniaxial anisotropy energy, and the interlayer coupling energy of bi-linear type. The magnetic moments of the FM layers, $\mathbf{M}_1$ = ($M$, $\varphi_1$) and $\mathbf{M}_2$ = ($M$, $\varphi_2$), are of the same magnitude, as illustrated in Fig. C1. $B_\mathrm{a}$ and $B_j$ are effective fields of uniaxial (two-fold) anisotropy and bi-linear interlayer coupling, respectively. Converting to angular variables $\varphi = (\varphi_1 + \varphi_2)/2$ and $\Delta\varphi = (\varphi_1 - \varphi_2)$ simplifies the expression for the magnetic free energy of the system to

$$U = -2MB\cos(\varphi - \varphi_B)\cos\Delta\varphi/2 - 1/2\, MB_\mathrm{a}\cos 2\varphi\cos\Delta\varphi + 1/2\, MB_j\cos\Delta\varphi. \tag{C2}$$

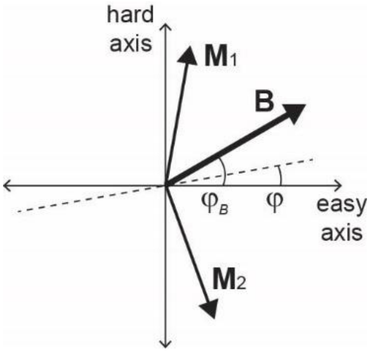


**Figure C1.** Reference-frame schematic of in-plane $\mathbf{M}_1$, $\mathbf{M}_2$, and **B** with respect to the easy axis of two-fold magnetic anisotropy of a nano-crystallite.

*M*(*B*) is obtained by finding parameters ($\varphi$, $\Delta\varphi$), which correspond to the minimum of *U* (Eq. C2) for given ($\varphi_B$, $B_\mathrm{a}$, $B_j$), according to

$$M/M_\mathrm{s} = \left[\cos(\varphi_1 - \varphi_B) + \cos(\varphi_2 - \varphi_B)\right]/2 = \cos(\varphi - \varphi_B)\cos(\Delta\varphi/2). \tag{C3}$$

Epitaxial (100) Fe based multilayers grown on single-crystal substrates are usually characterized by four-fold in-plane magnetic anisotropy [U. Köbler et al. *J. Magn. Magn. Mater.* **103** (1992) 236], while substrates of other texture [e.g., (211)] can result in two-fold anisotropy [M. Grimsditch, S. Kumar, and E. E. Fullerton, *Phys. Rev. B* **54** (1996) 3385]. The main difference in M(B) between the two cases is in the presence of two characteristic steps in M vs. B when the anisotropy is four-fold and only one M-vs-B step when it is two-fold. Our additional VSM and FMR studies of the reference Fe(2 nm) films and Fe/Cr/Fe tri-layers (not included herein) did not reveal any significant in-plane angular dependence in the hysteresis loops or resonance spectra, leading us to conclude that essentially no *macroscopic* in-plane magnetic anisotropy is present. On the other hand, the numerical analysis described above concludes that the measured one-step-shaped $M(B)$ loops for the RKKY-coupled Fe/Cr/Fe trilayers must be due to two-fold magnetic anisotropy on the scale of the individual crystallites forming the polycrystalline films. Assuming uniform angular distribution of the local anisotropy easy axes in the film plane, expected in our case of deposition on rotating substrates, provides an excellent agreement between the model and the experimental data. Such pattern of magnetic anisotropy has been explained in terms of polycrystalline nature of the sputtered multilayers and in-plain strain variations between the nano-crystalline grains [M. T. Johnson et al. Magnetic anisotropy in metallic multilayers, *Rep. Prog. Phys.* **59** (1996) 1409]. A more detailed study of the magnetic anisotropy in the present films goes beyond the scope of this paper and is outside its main focus. Regardless of the details of the intrinsic anisotropy in our Fe films, the model-extraction of the interlayer coupling is quite robust and, together with the zero remnance observed under RKKY coupling, clearly point to strong antiferromagnetic RKKY in the system, highly efficiently controlled by temperature.
